# Supplementary material for: Generative AI-Downscaling of Large Ensembles Project Unprecedented Future Droughts
Source: arXiv:2509.21844 source file (2025-09-26)
Supplement: Supplementary file 1 [file Supplementary_Material_drought.pdf]

# Supplementary Material for: Generative AI Downscaling of Large Ensembles Project Unprecedented Future Droughts

Hamish Lewis<sup>1,2\*</sup>, Neelesh Rampal<sup>2,3,4</sup>, Peter B. Gibson<sup>2</sup>,  
Luke J. Harrington<sup>1</sup>, Chiara M. Holgate<sup>5,6</sup>, Anna Ukkola<sup>3,4</sup>,  
Nicola M. Maher<sup>5,6</sup>

<sup>1</sup>School of Science, University of Waikato, Hamilton, New Zealand.

<sup>2</sup>Earth Sciences New Zealand, New Zealand.

<sup>3</sup>ARC Centre of Excellence for Weather of the 21st Century, University  
of New South Wales, Sydney, Australia.

<sup>4</sup>Climate Change Research Centre, University of New South Wales,  
Sydney, Australia.

<sup>5</sup>Research School of Earth Sciences, Australian National University,  
Canberra, Australia.

<sup>6</sup>ARC Centre of Excellence for the Weather of the 21st Century,  
Australian National University, Canberra, Australia.

\*Corresponding author(s). E-mail(s): [hamish.lewis@waikato.ac.nz](mailto:hamish.lewis@waikato.ac.nz);  
Contributing authors: [neelesh.rampal@niwa.co.nz](mailto:neelesh.rampal@niwa.co.nz);  
[peter.gibson@niwa.co.nz](mailto:peter.gibson@niwa.co.nz); [luke.harrington@waikato.ac.nz](mailto:luke.harrington@waikato.ac.nz);  
[chiara.holgate@anu.edu.au](mailto:chiara.holgate@anu.edu.au); [a.ukkola@unsw.edu.au](mailto:a.ukkola@unsw.edu.au);  
[nicola.maher@anu.edu.au](mailto:nicola.maher@anu.edu.au);

## Contents

S1-S2: Added value breakdown of annual precip within ACCESS-CM2 and NorESM2-MM

S3-S4: Comparison of climate change signal of drought duration and frequency within GCM, RCM, and AI outputs

S5-S7: Projections of seasonal precipitation across ensembles

S8-S12: Projections of drought and precipitation metrics for the members of the CanESM5 ensemble.

S13-S17: Projections of drought and precipitation metrics for the members of the ACCESS-ESM1-5 ensemble.

S17-S22: Projections of drought and precipitation metrics for the other CMIP6 GCMs used in this study.

S23-S27: Projections of drought and precipitation metrics for the models dynamically downscaled with CCAM.

S28: Longest droughts present in the VCSN dataset and ERA5 downscaled with CCAM.

S29: Longest droughts in the ACCESS-ESM1-5 ensemble using various subsample sizes.

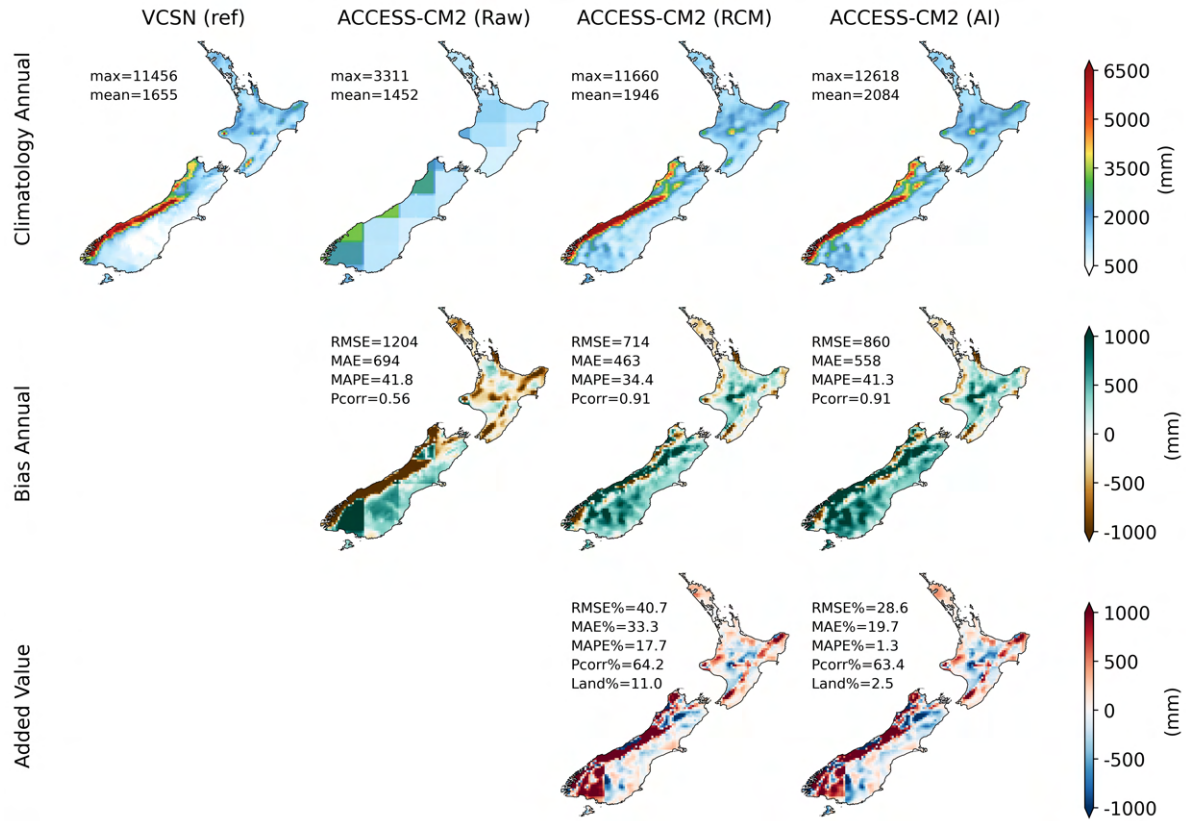

**Fig. S1** Added value for the annual mean precipitation climatology (1985-2014) through downscaling the ACCESS-CM2 GCM with the CCAM RCM and generative AI. The top row shows the climatology of each dataset. The middle row shows the absolute biases between each dataset and the VCSN reference dataset, with the error metrics of each dataset shown. The bottom row shows the added value of RCM (bottom left) and AI (bottom right) downscaling, where positive values (red) indicate a reduction in absolute biases. Improvements in error metrics as percentages averaged across the land surface are also shown.

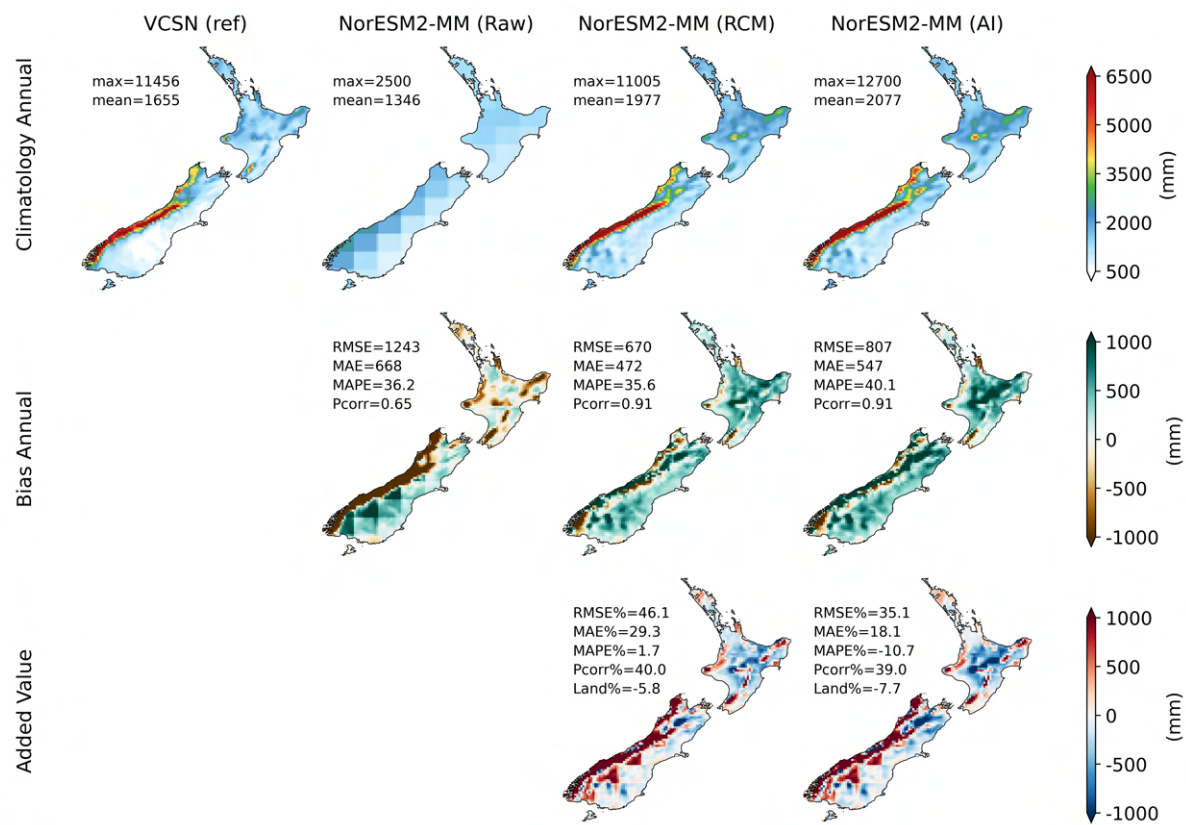

**Fig. S2** The same as Figure S1, but for NorESM2-MM.



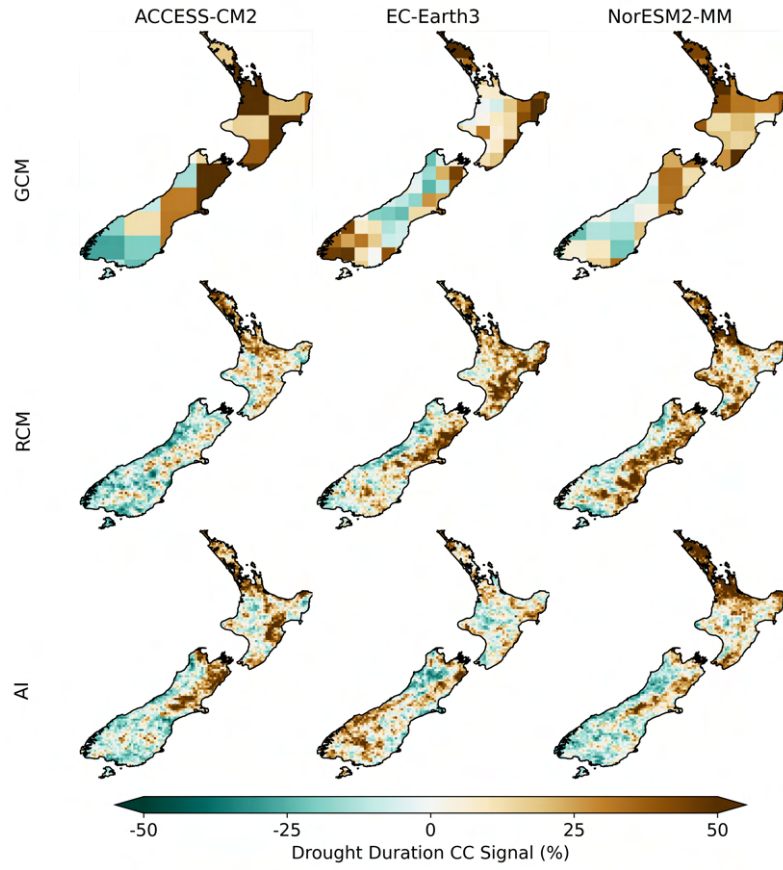

**Fig. S3** Climate change signal of meteorological drought duration between 2070-2099 in SSP3-7.0 relative to 1985-2014 in historical simulations. The rows show the climate change signal within the GCM, downscaled RCM output, and AI downscaled output respectively, while the columns show the host GCMs: ACCESS-CM2, EC-Earth3, and NorESM2-MM.

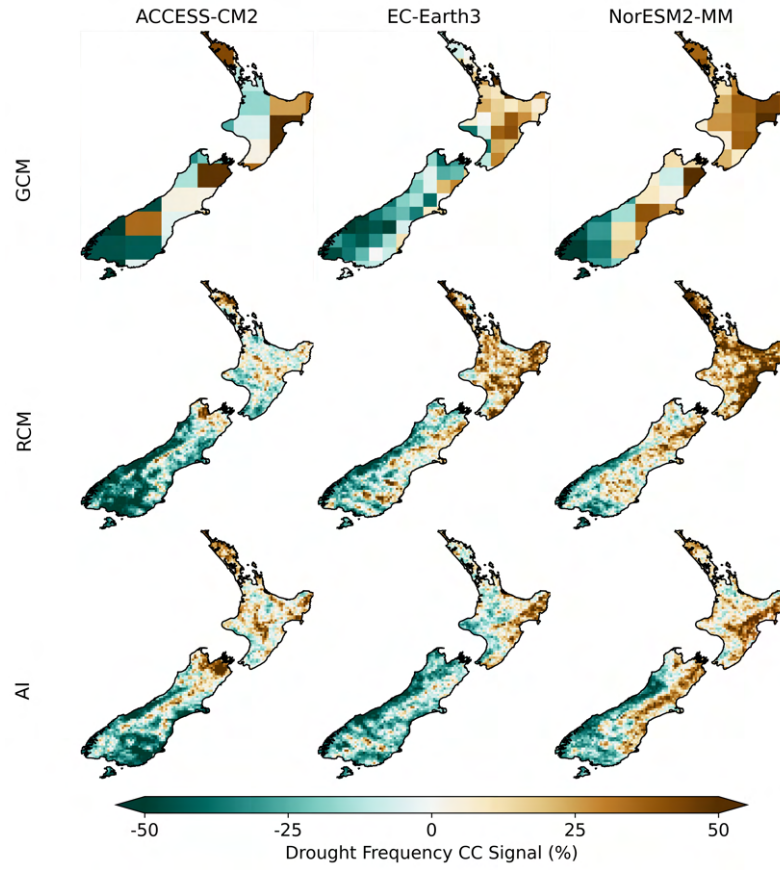

**Fig. S4** Climate change signal of meteorological drought frequency between 2070-2099 in SSP3-7.0 relative to 1985-2014 in historical simulations. The rows show the climate change signal within the GCM, downscaled RCM output, and AI downscaled output respectively, while the columns show the host GCMs: ACCESS-CM2, EC-Earth3, and NorESM2-MM.

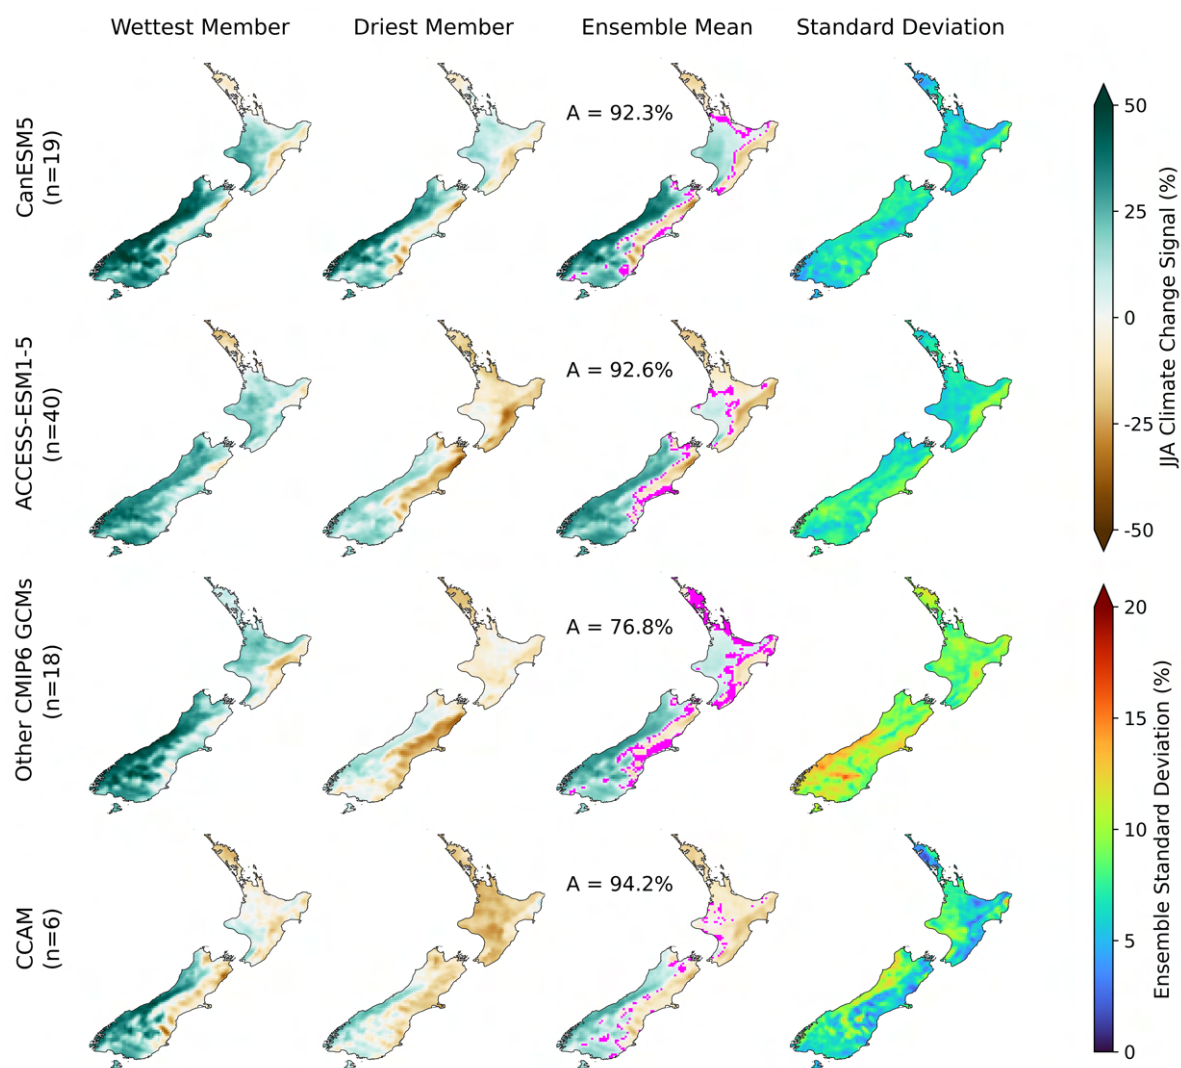

**Fig. S5** JJA precipitation climate change signal between in 2070-2099 in SSP3-7.0 compared to 1985-2014 in historical simulations. The columns show the wettest member, driest member, ensemble mean, and inter-member standard deviation of each ensemble: CanESM5, ACCESS-ESM1-5, all other CMIP6 GCMs, and CCAM downscaled GCMs, which constitute the rows. Pink coloring of the ensemble means denotes grid-points where less than 66% of ensemble members agree on the sign of change. The percentage of the land surface over which the ensemble agrees on the sign of change (A) is presented alongside the ensemble means.

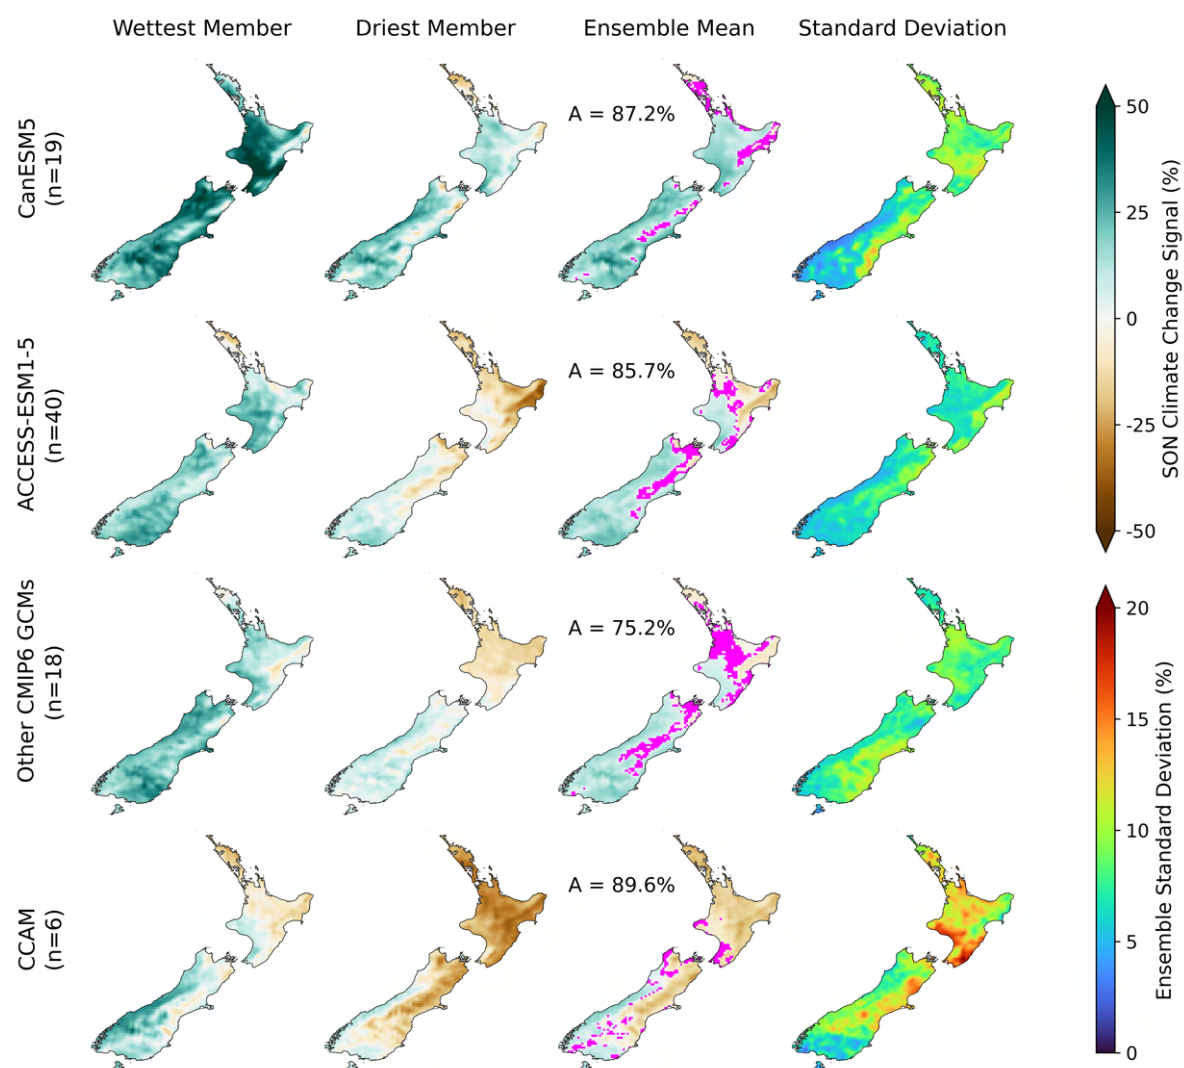

**Fig. S6** The Same as Figure S5, but for SON.

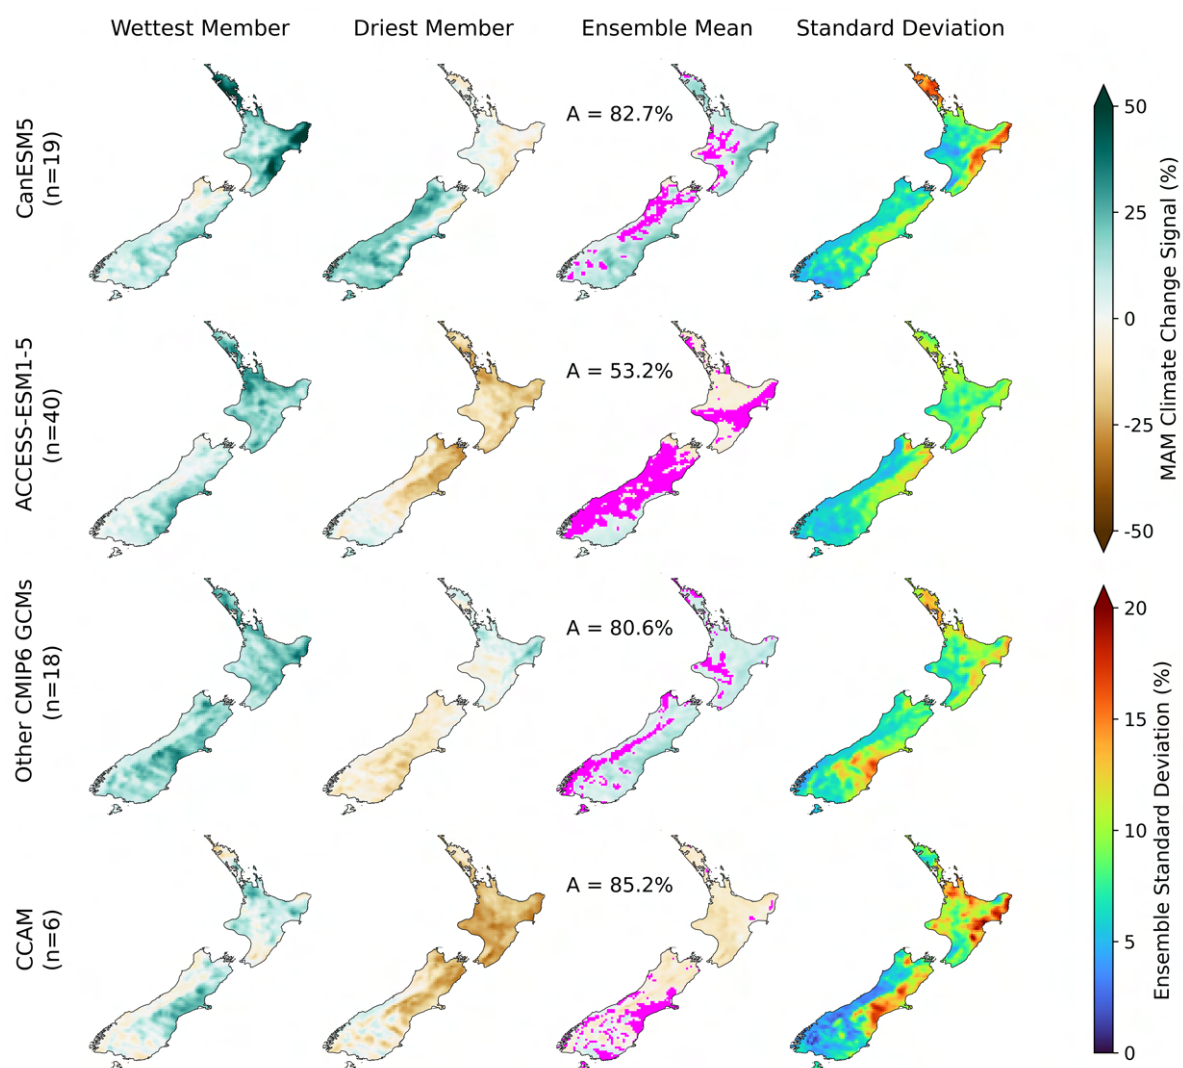

**Fig. S7** The Same as Figure S5, but for MAM.

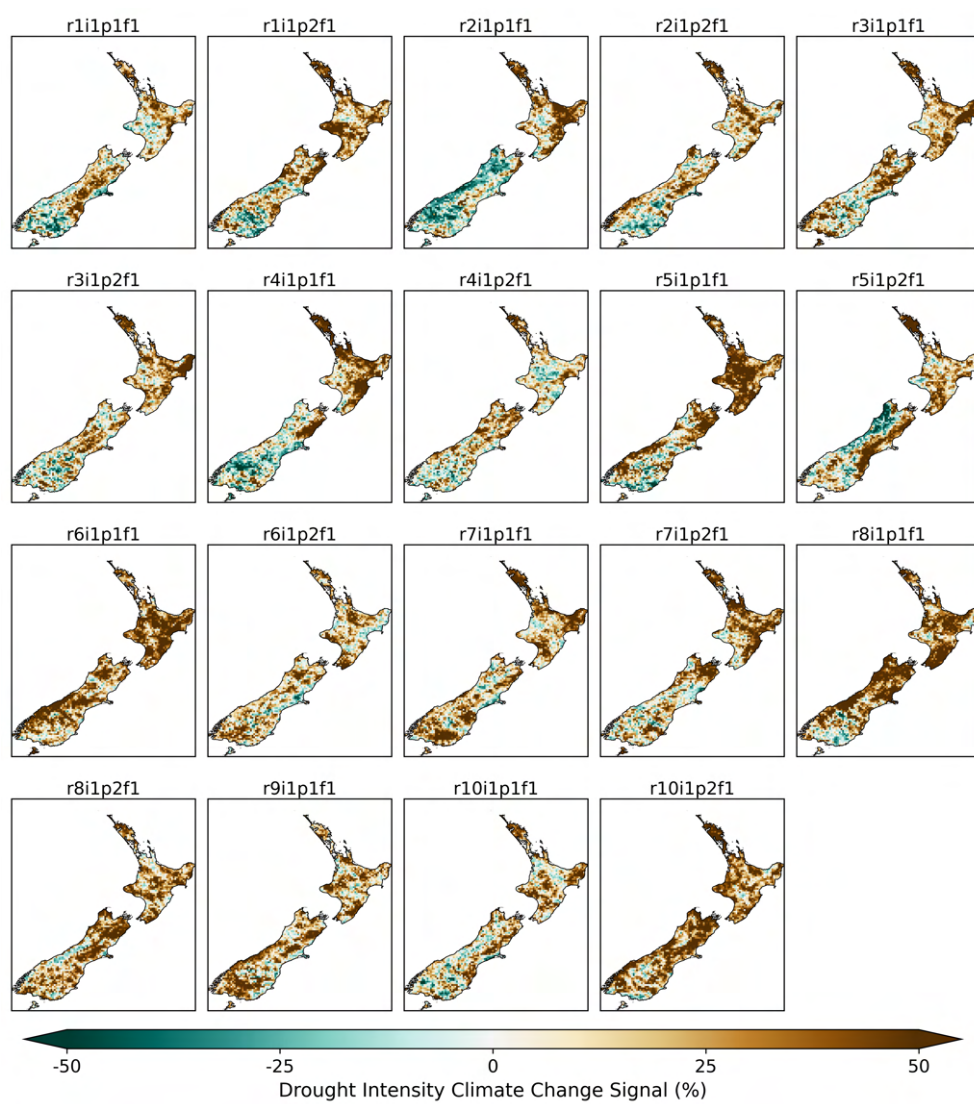

**Fig. S8** Climate change signal of drought intensity for the members of CanESM5.



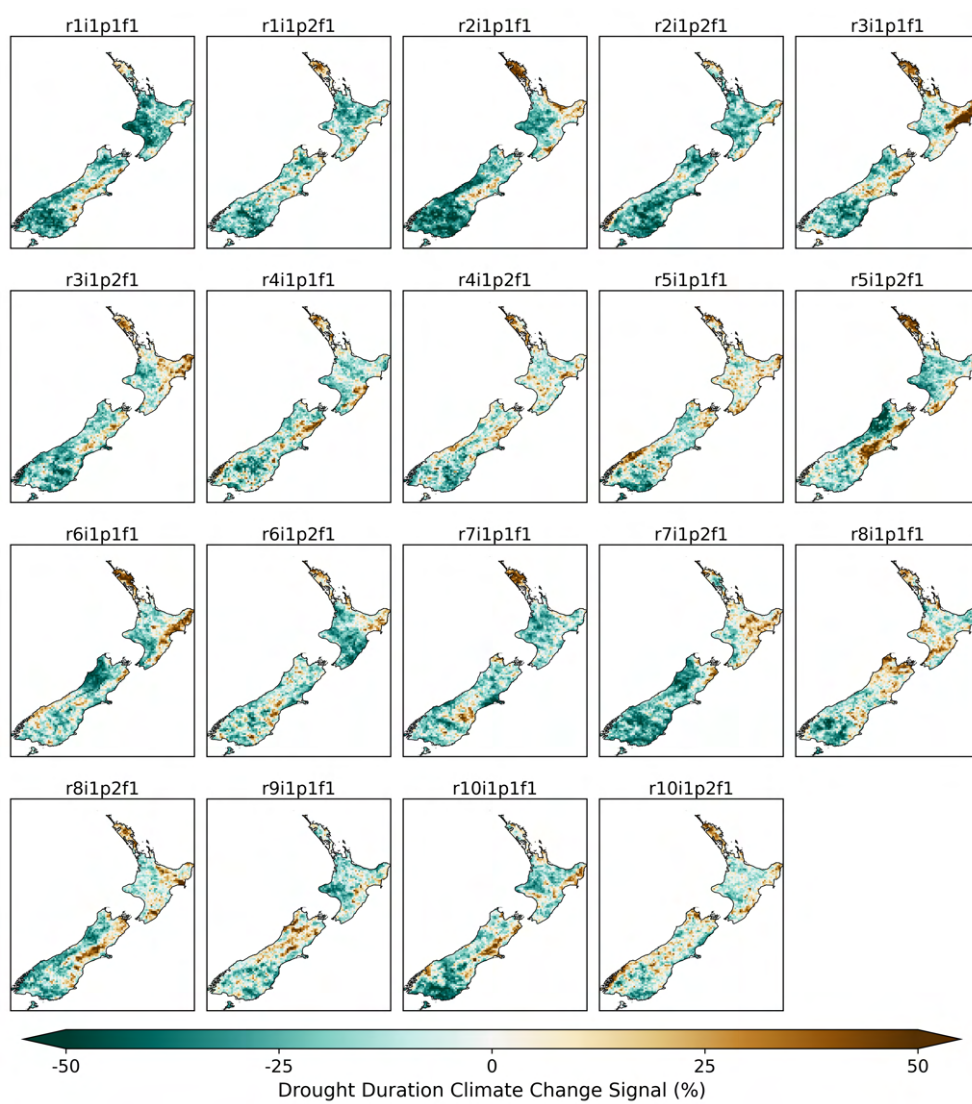

**Fig. S9** Climate change signal of drought duration for the members of CanESM5.

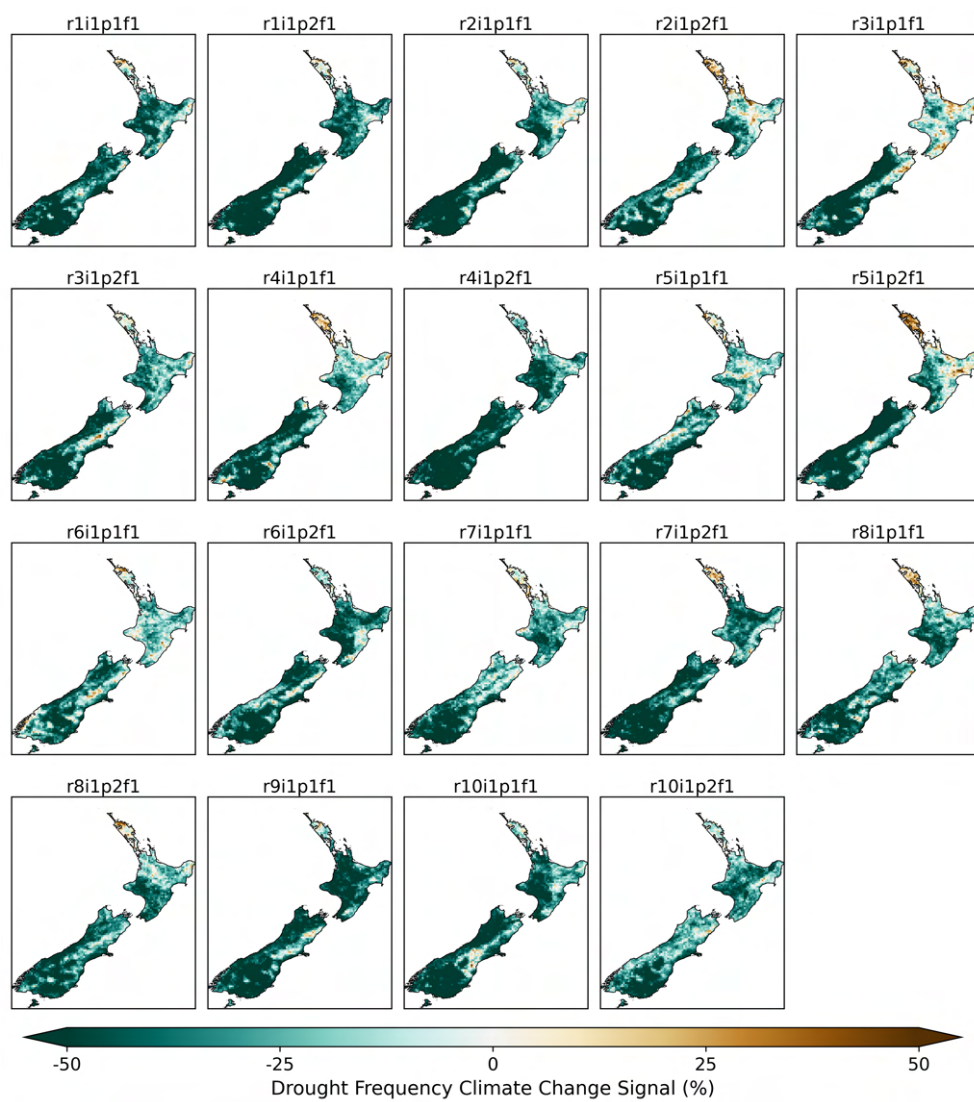

**Fig. S10** Climate change signal of drought frequency for the members of CanESM5.



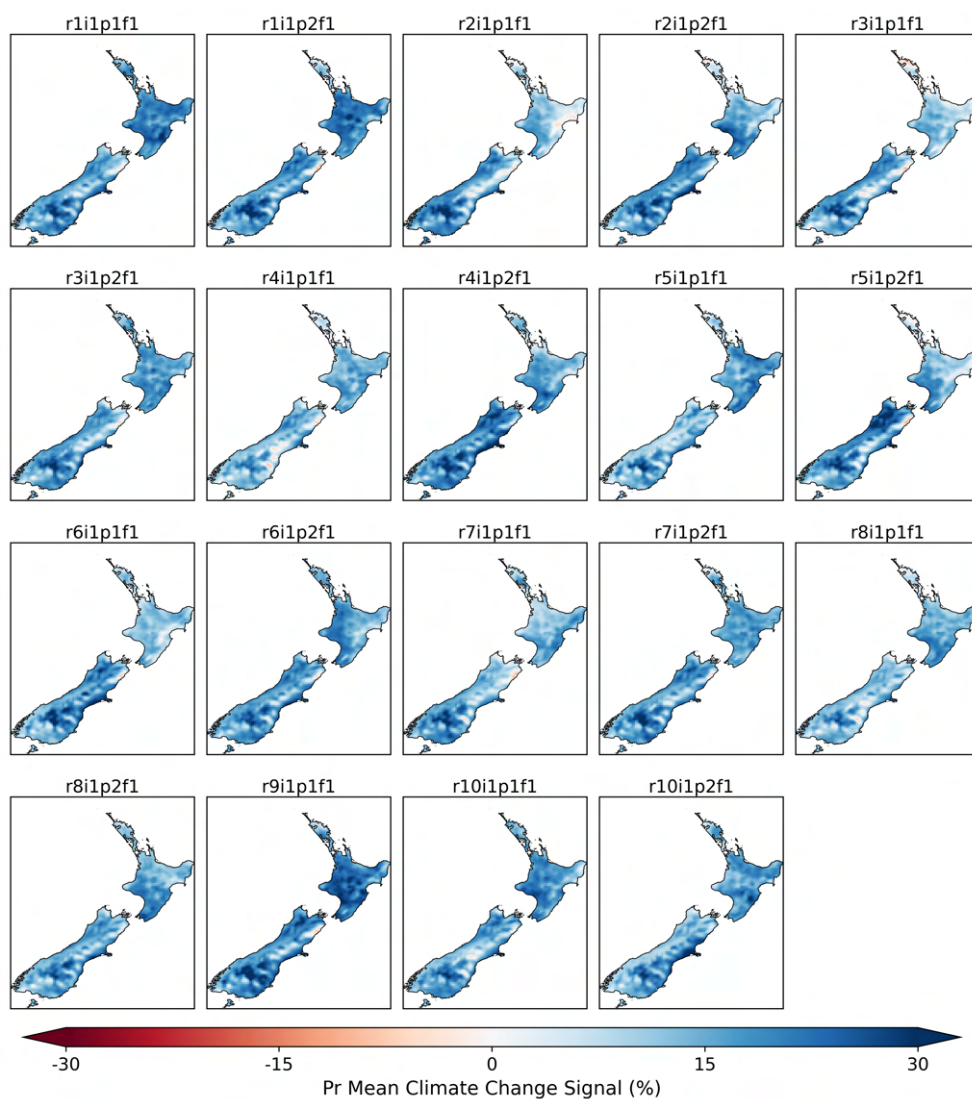

**Fig. S11** Climate change signal of annual mean precipitation for the members of CanESM5.

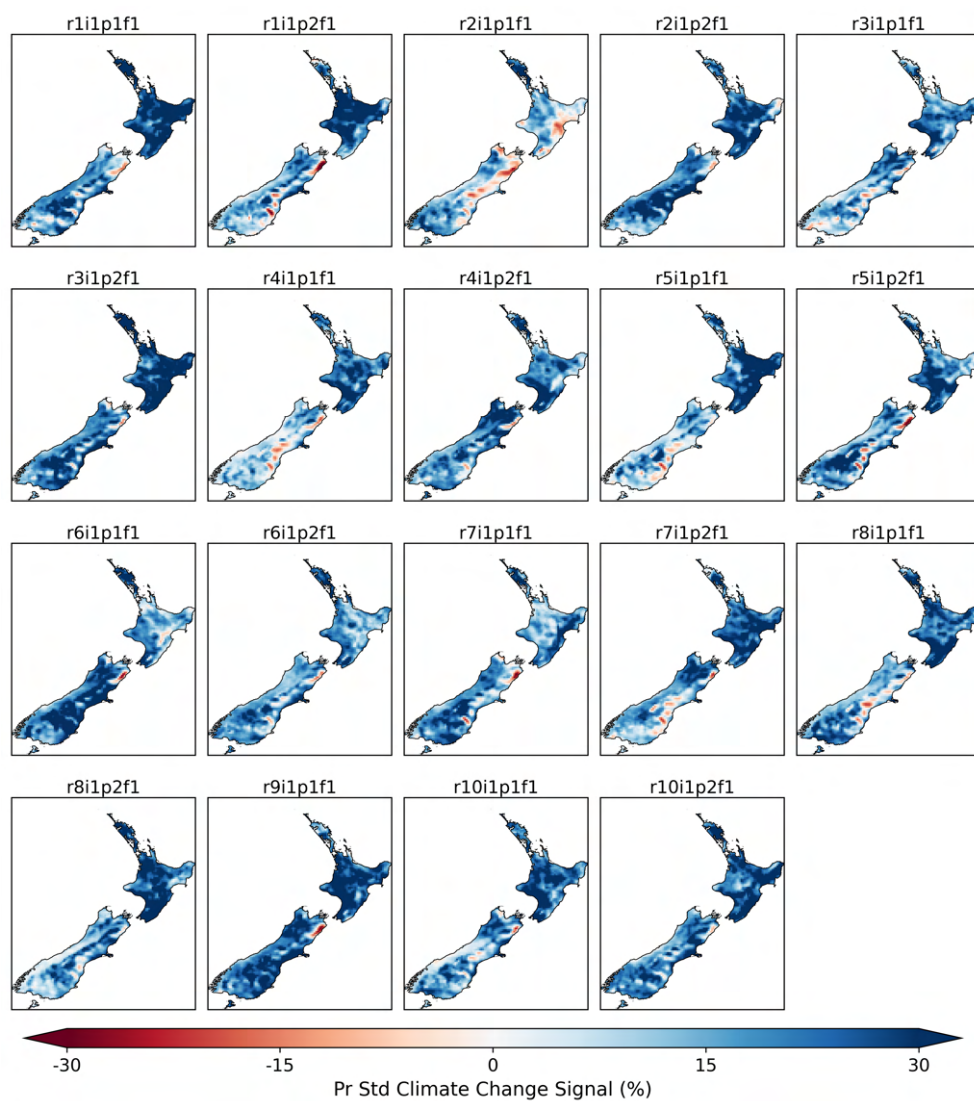

**Fig. S12** Climate change signal of month-to-month precipitation variability for the members of CanESM5.

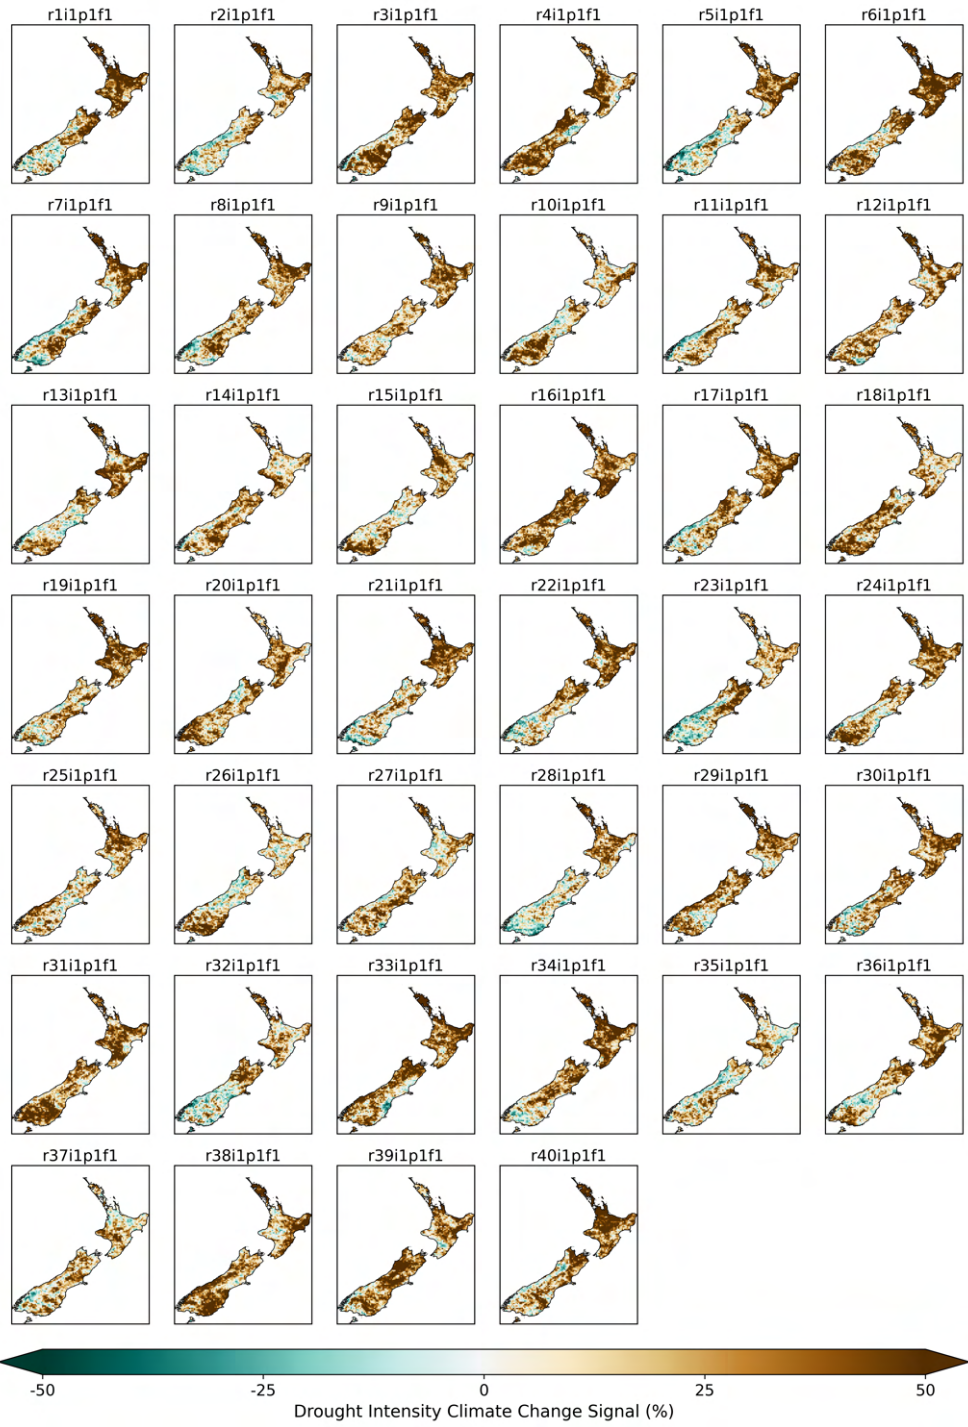

**Fig. S13** Climate change signal of drought intensity for the members of ACCESS-ESM1-5.

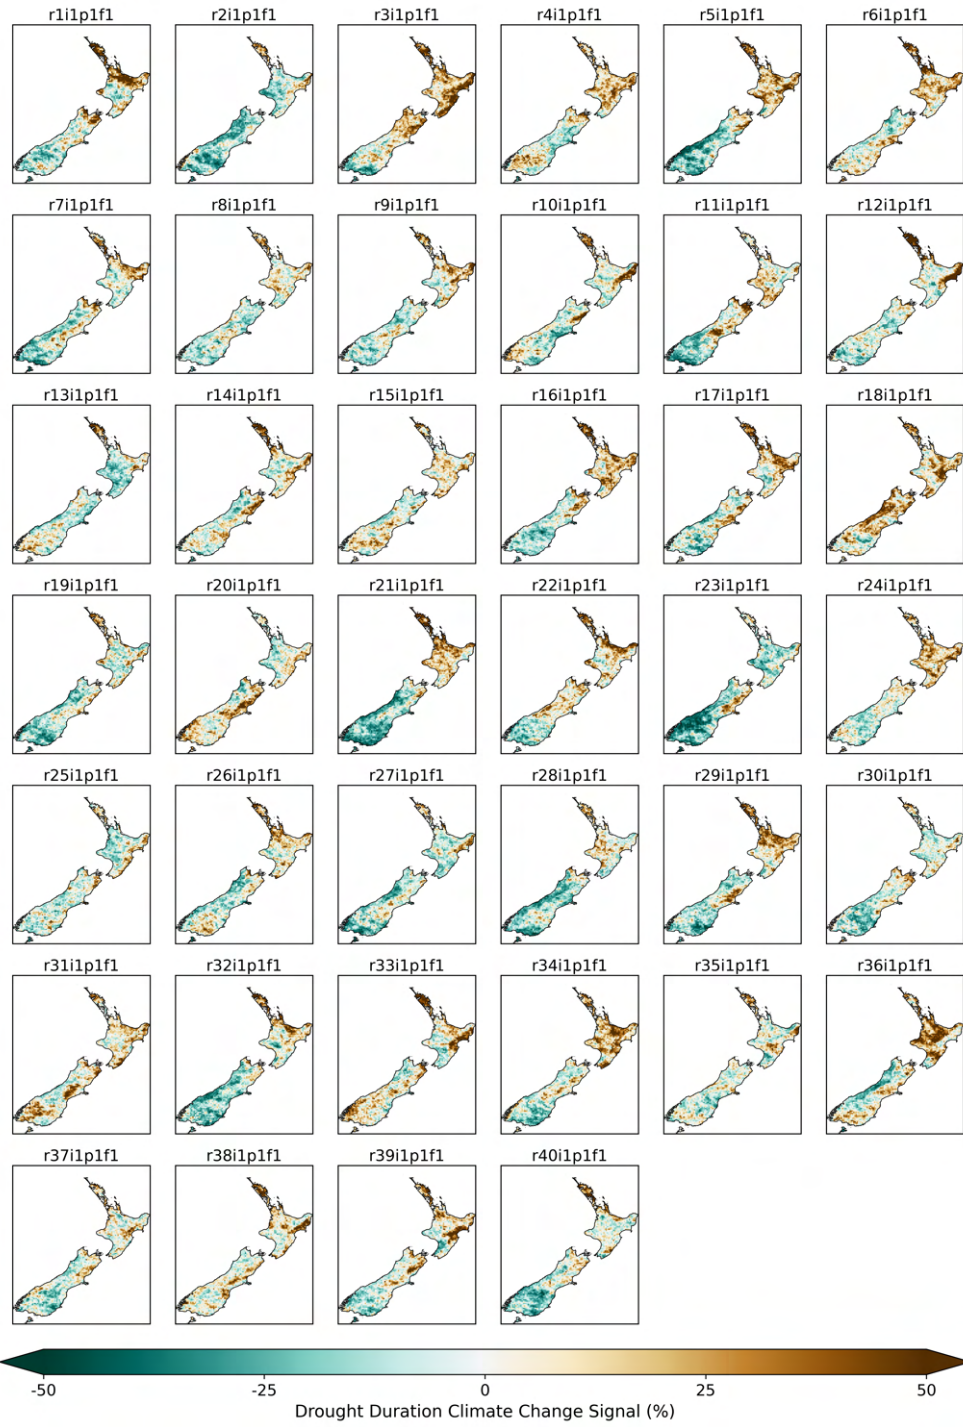

**Fig. S14** Climate change signal of drought duration for the members of ACCESS-ESM1-5.



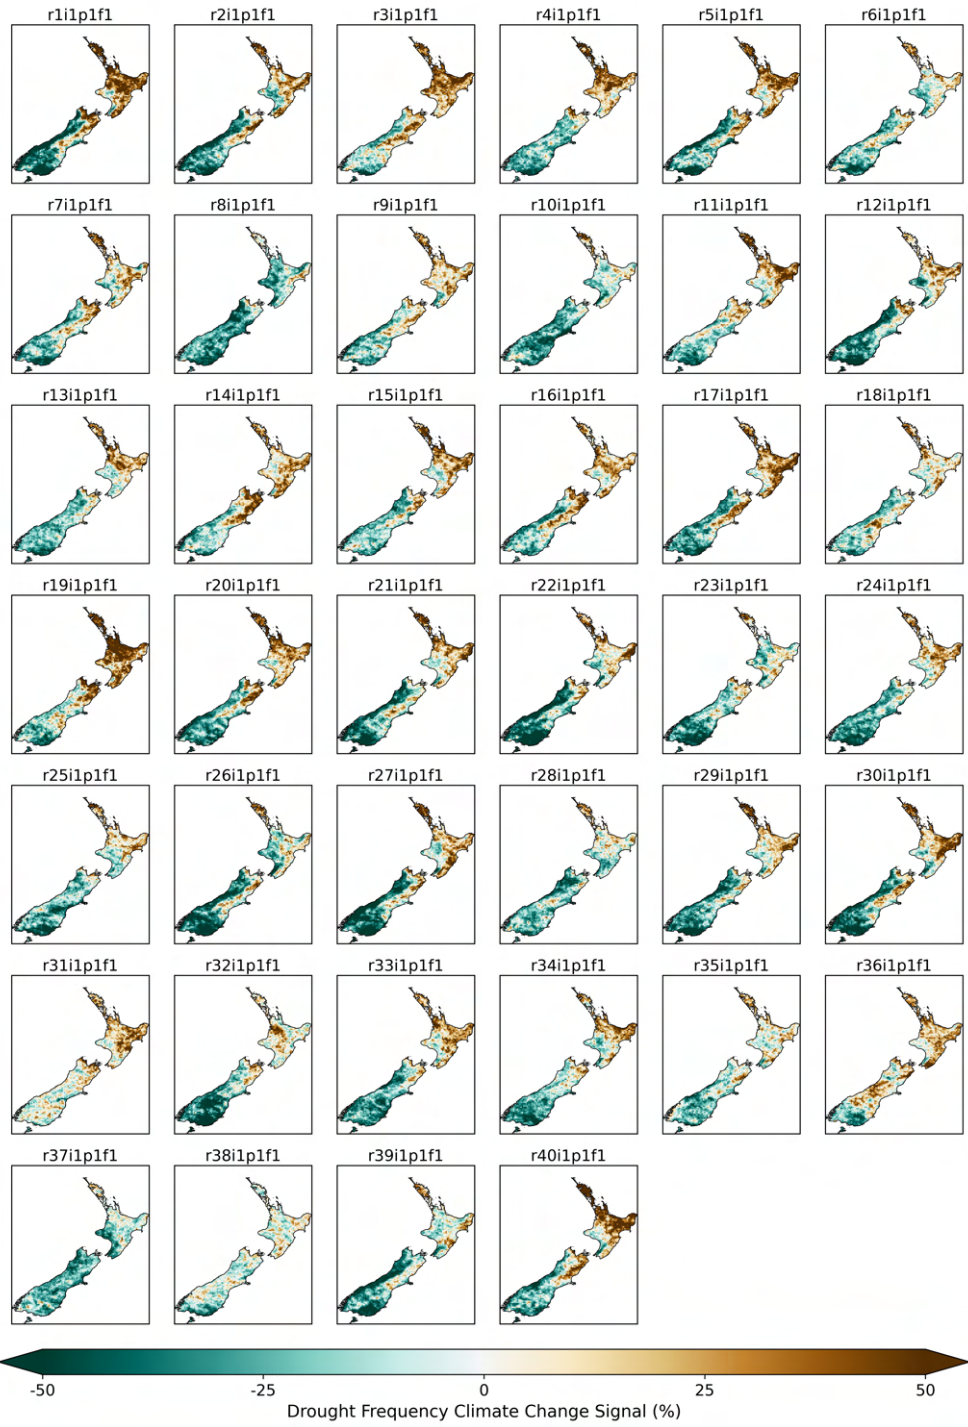

**Fig. S15** Climate change signal of drought frequency for the members of ACCESS-ESM1-5.

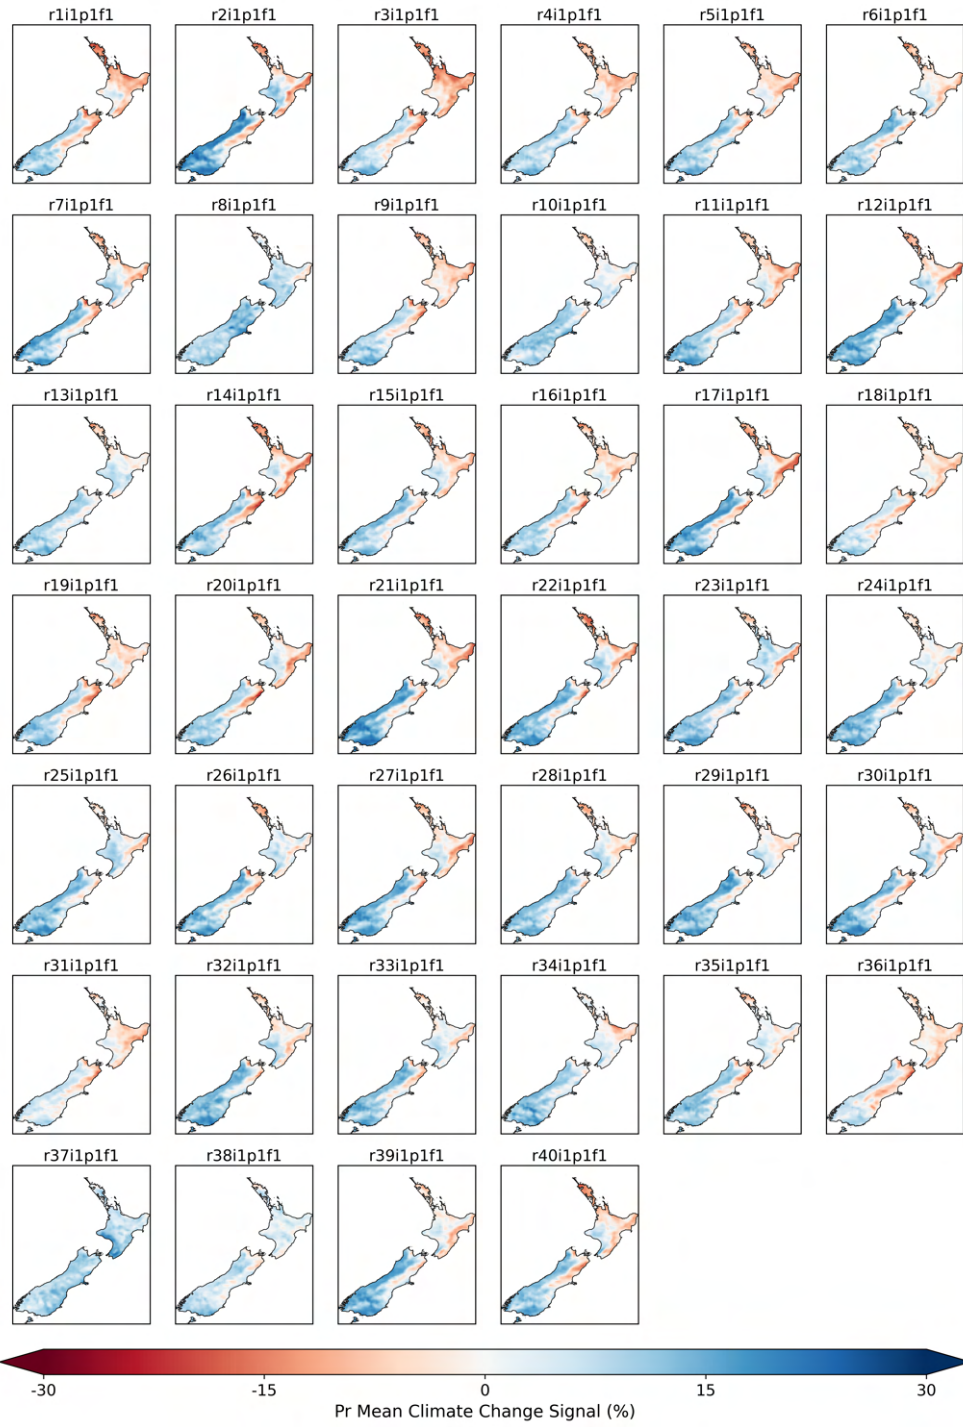

**Fig. S16** Climate change signal of annual mean precipitation for the members of ACCESS-ESM1-5.

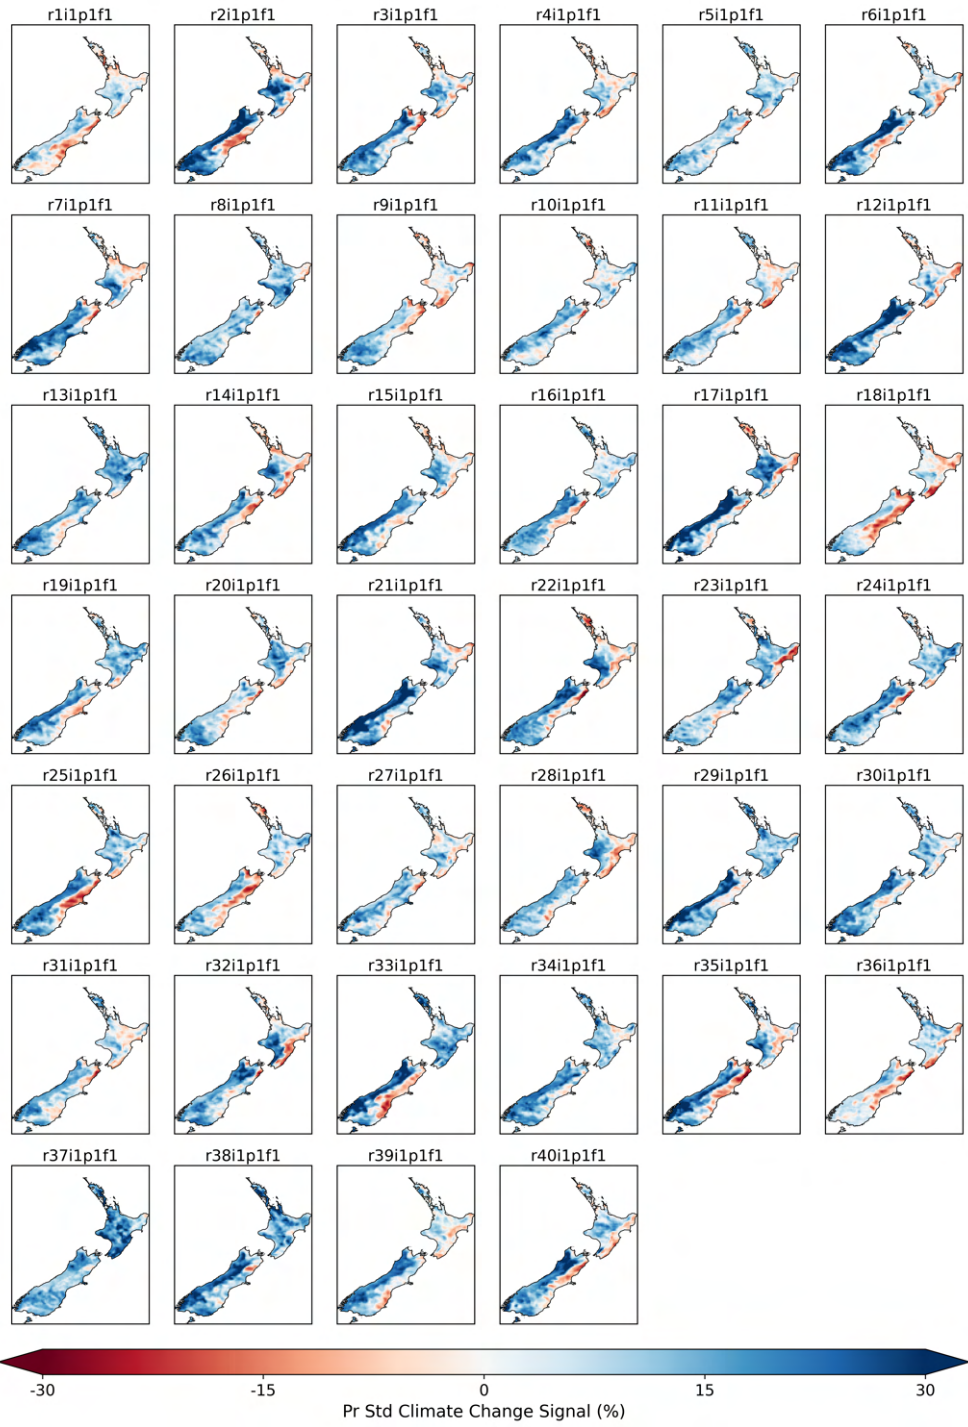

**Fig. S17** Climate change signal of month-to-month precipitation variability for the members of ACCESS-ESM1-5.

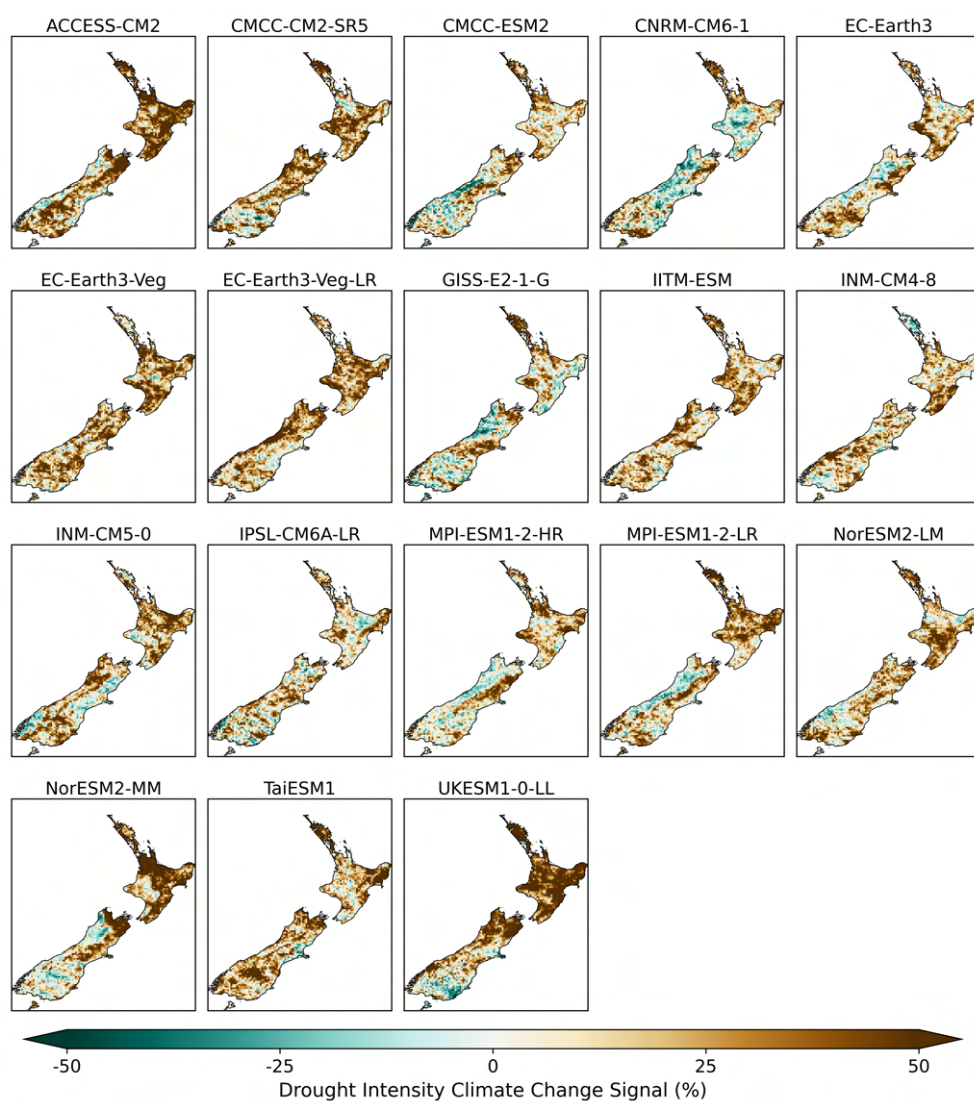

**Fig. S18** Climate change signal of drought intensity for the other CMIP6 GCMs used in this study.



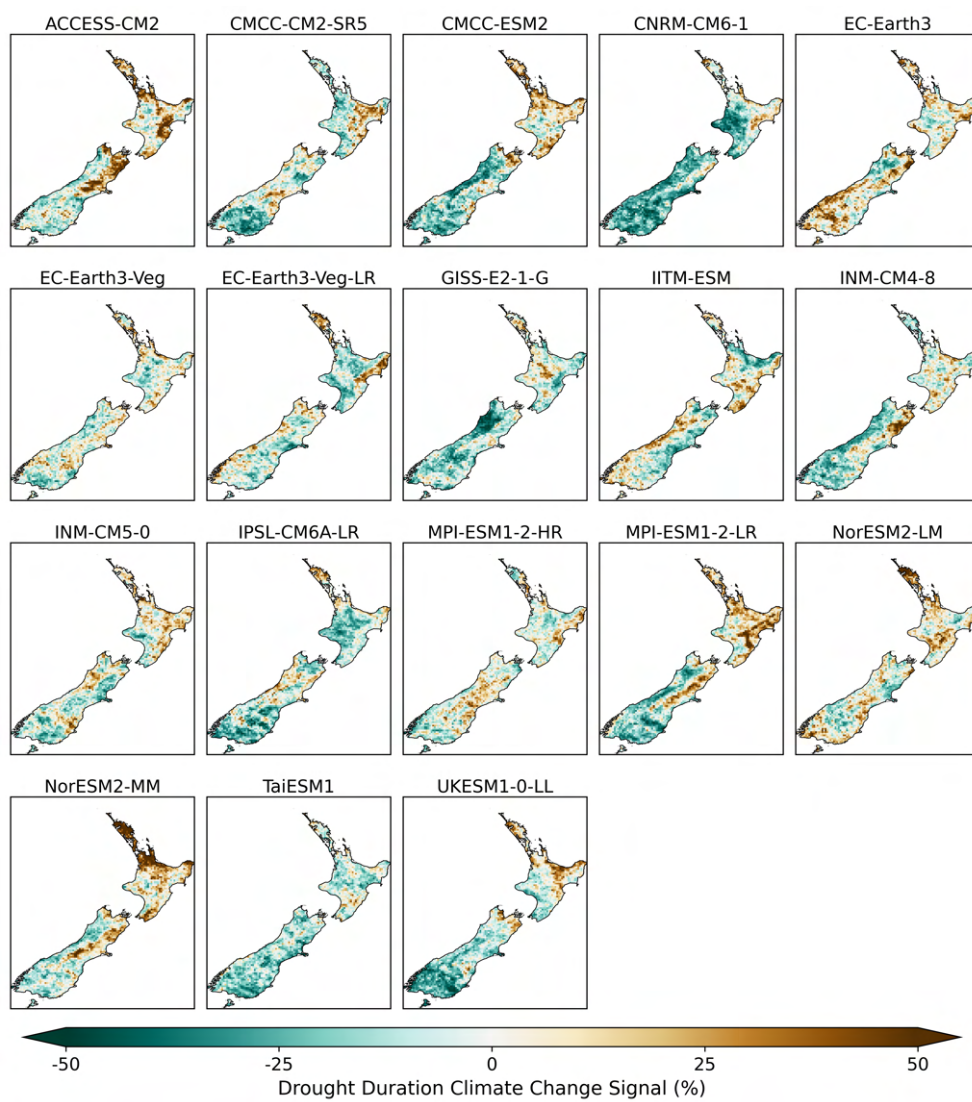

**Fig. S19** Climate change signal of drought duration for the other CMIP6 GCMs used in this study.

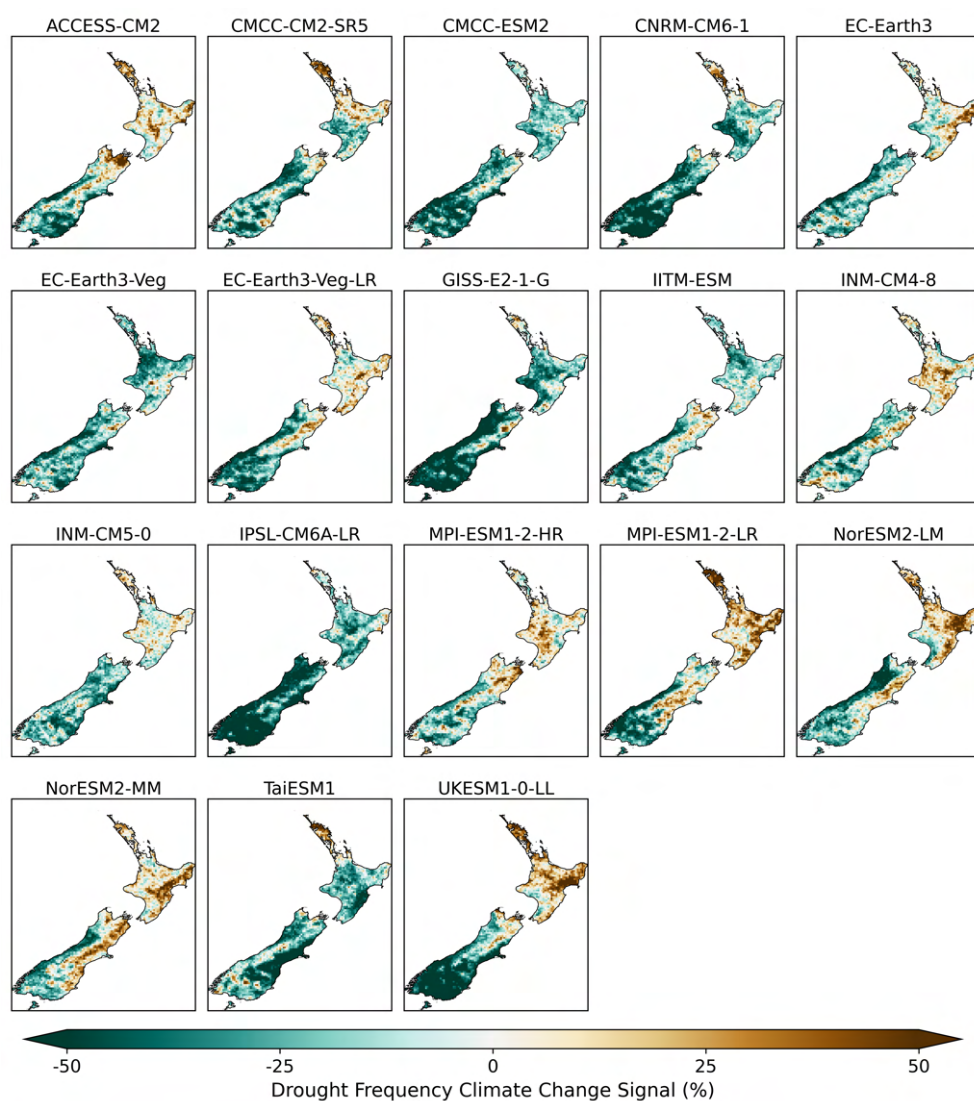

**Fig. S20** Climate change signal of drought frequency for the other CMIP6 GCMs used in this study.

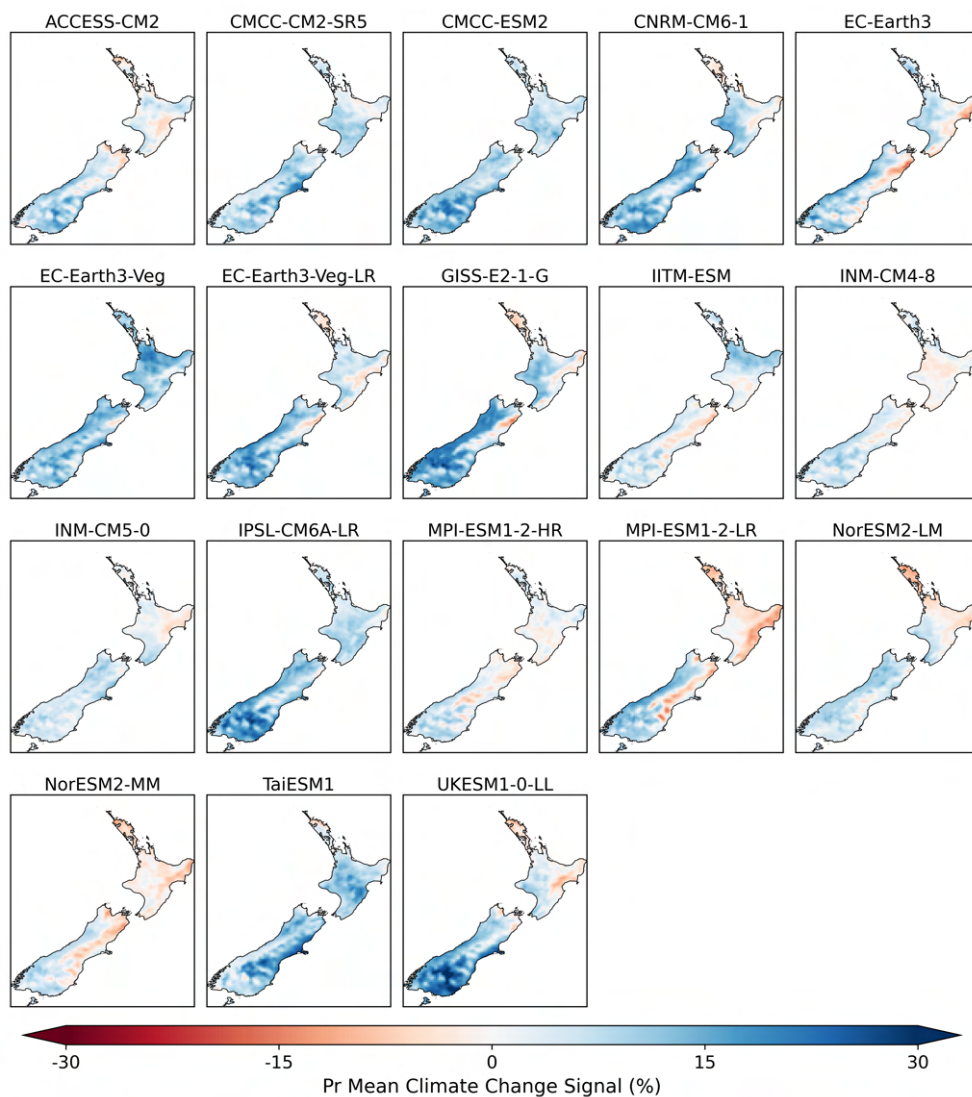

**Fig. S21** Climate change signal of annual mean precipitation for the other CMIP6 GCMs used in this study.

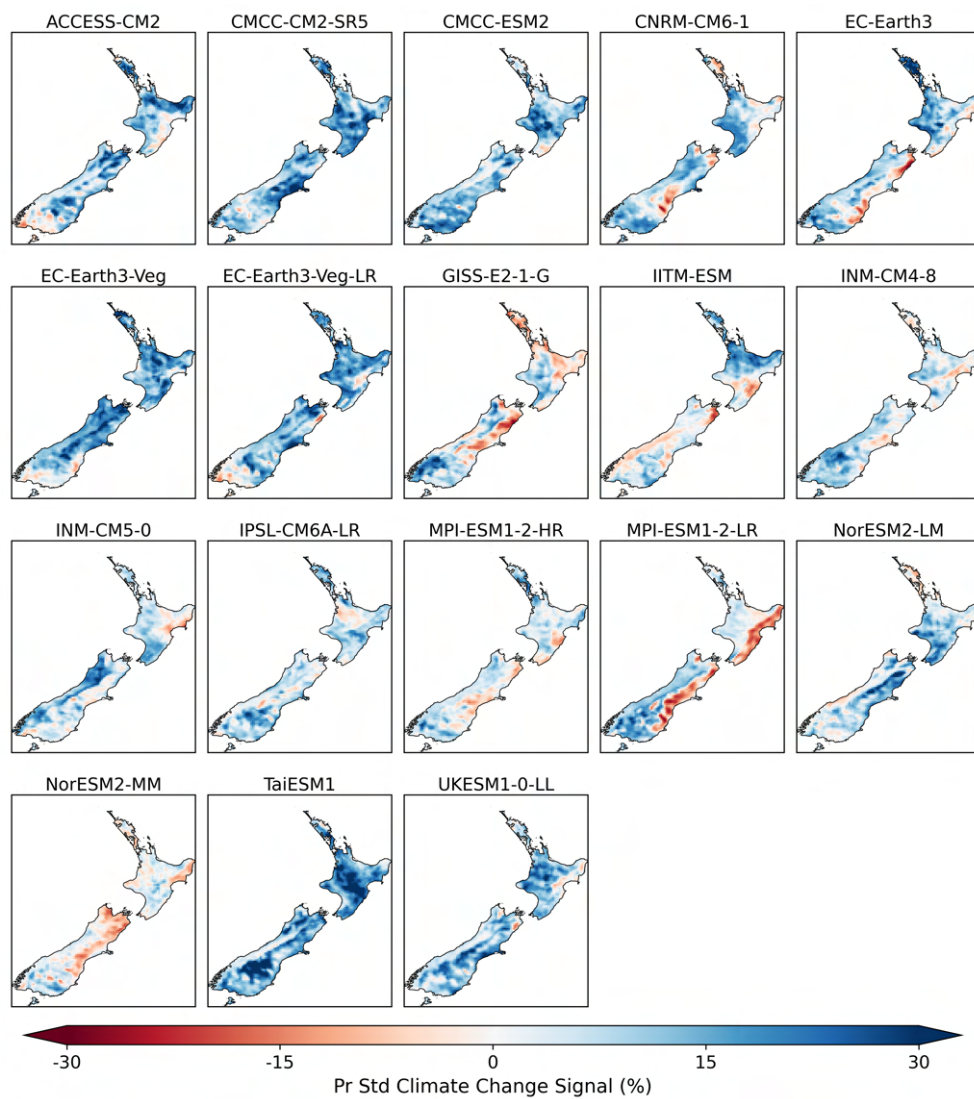

**Fig. S22** Climate change signal of month-to-month precipitation variability for the other CMIP6 GCMs used in this study.

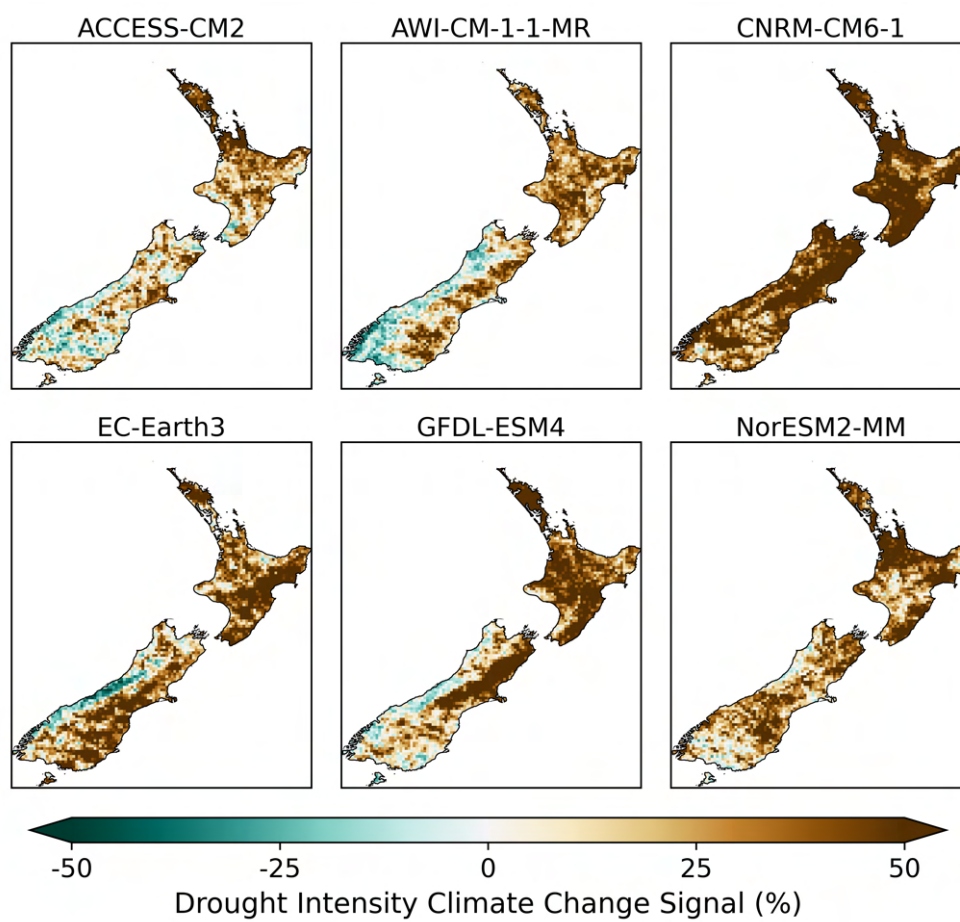

**Fig. S23** Climate change signal of drought intensity for the models dynamically downscaled with CCAM.

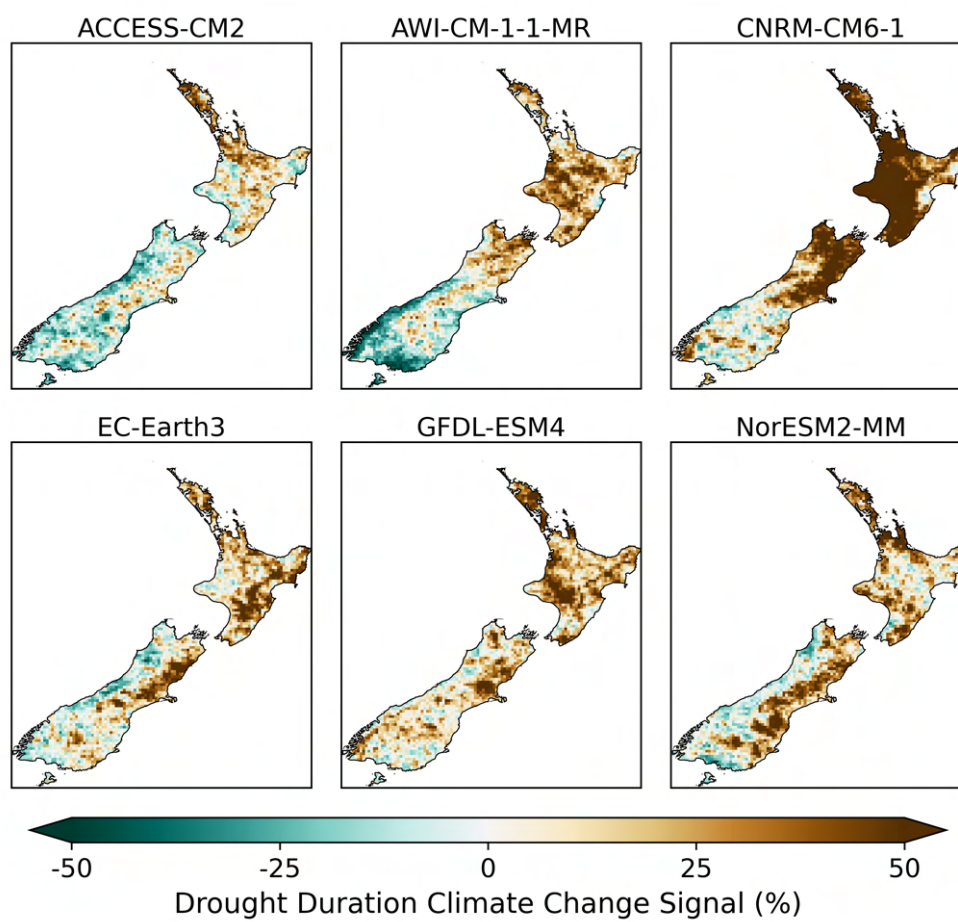

**Fig. S24** Climate change signal of drought duration for the models dynamically downscaled with CCAM.



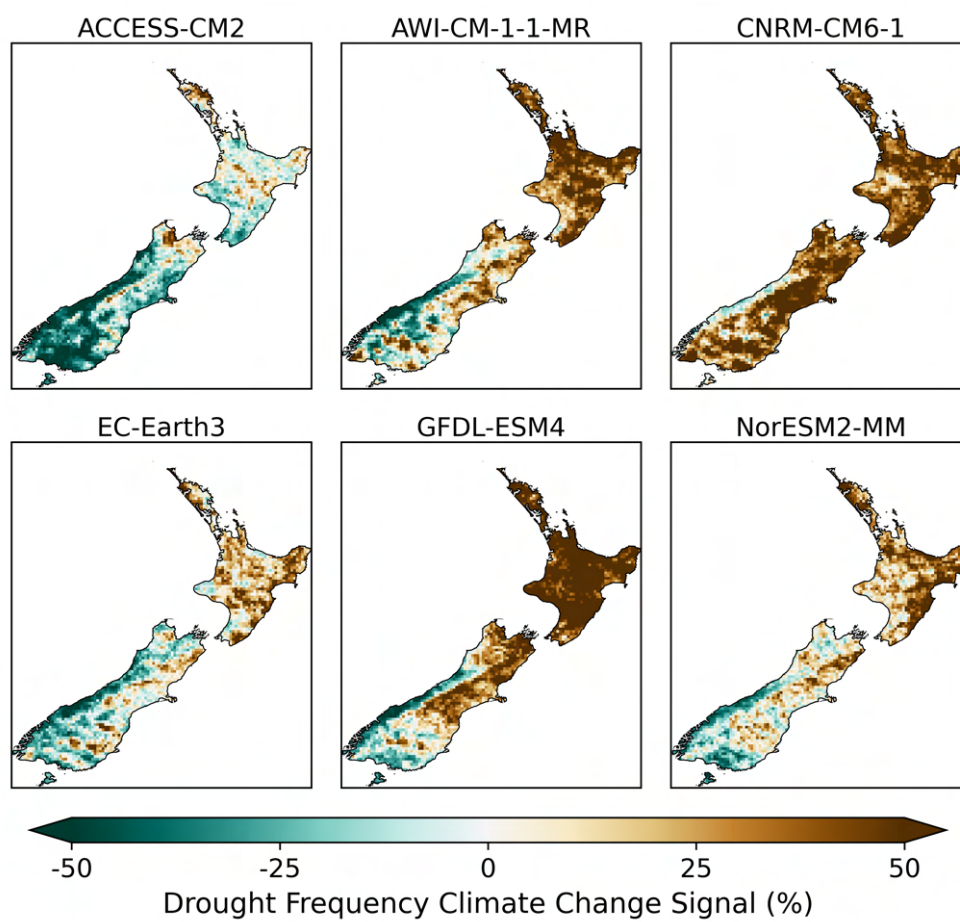

**Fig. S25** Climate change signal of drought frequency for the models dynamically downscaled with CCAM.

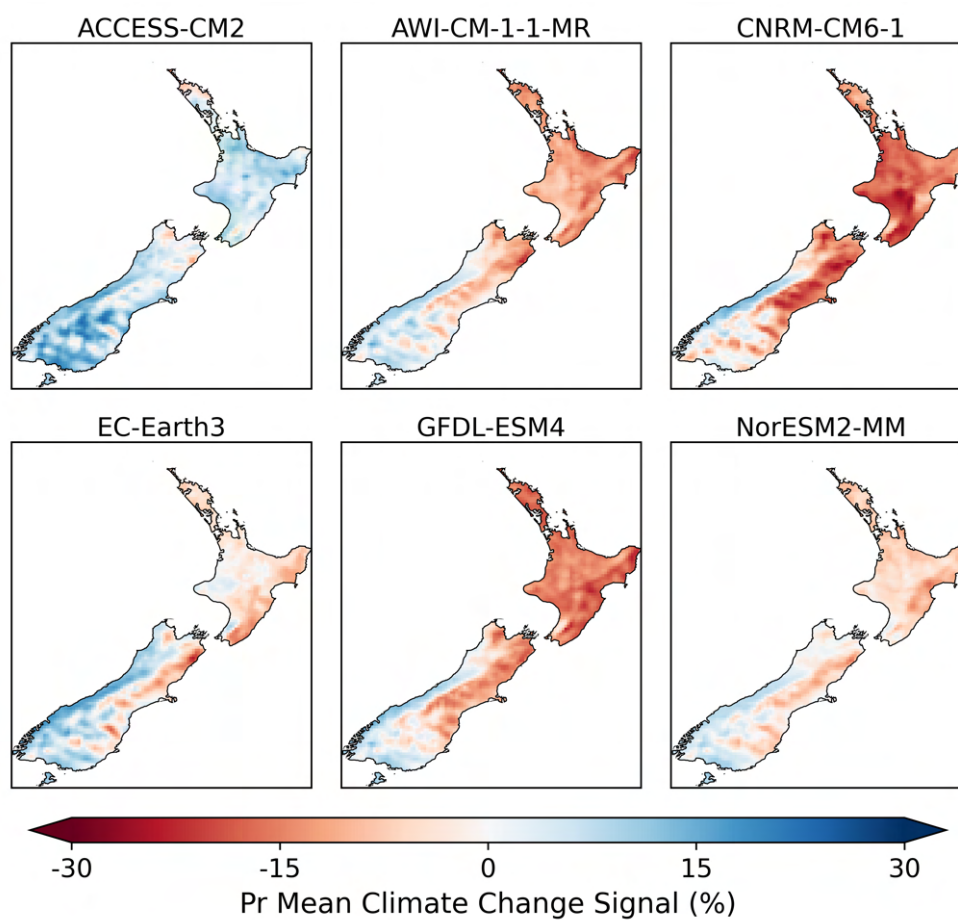

**Fig. S26** Climate change signal of annual mean precipitation for the models dynamically downscaled with CCAM.



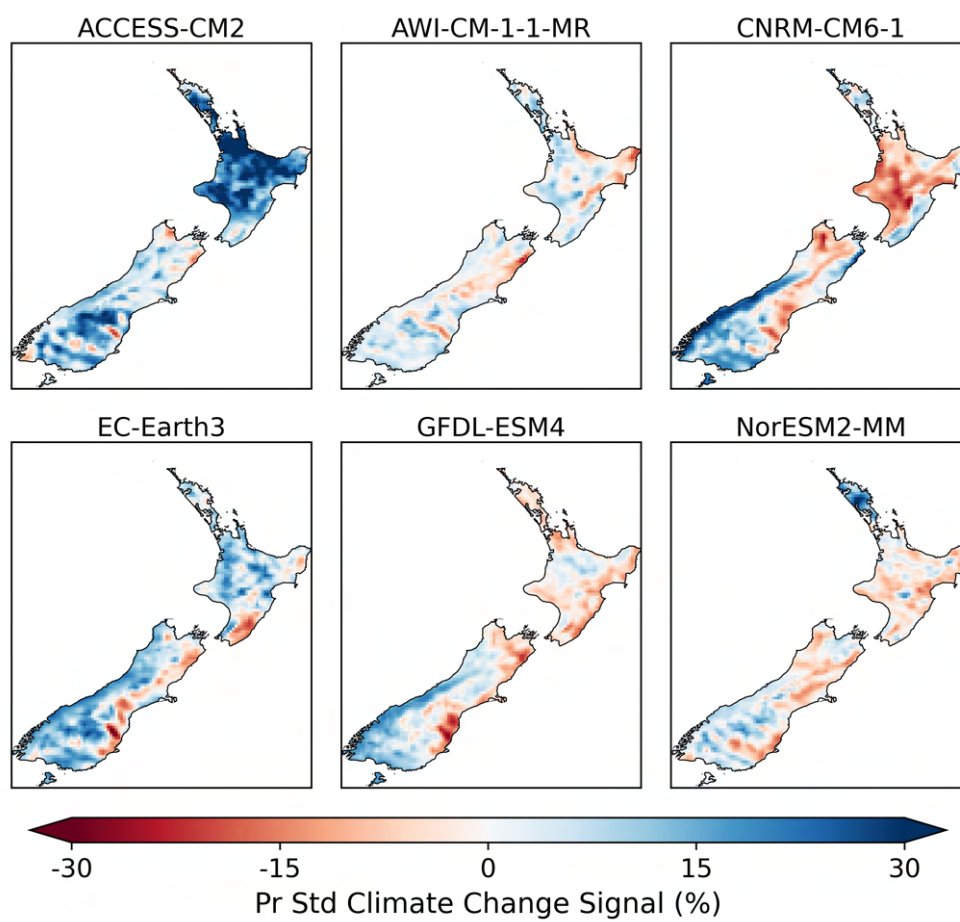

**Fig. S27** Climate change signal of month-to-month precipitation variability for the models dynamically downscaled with CCAM.

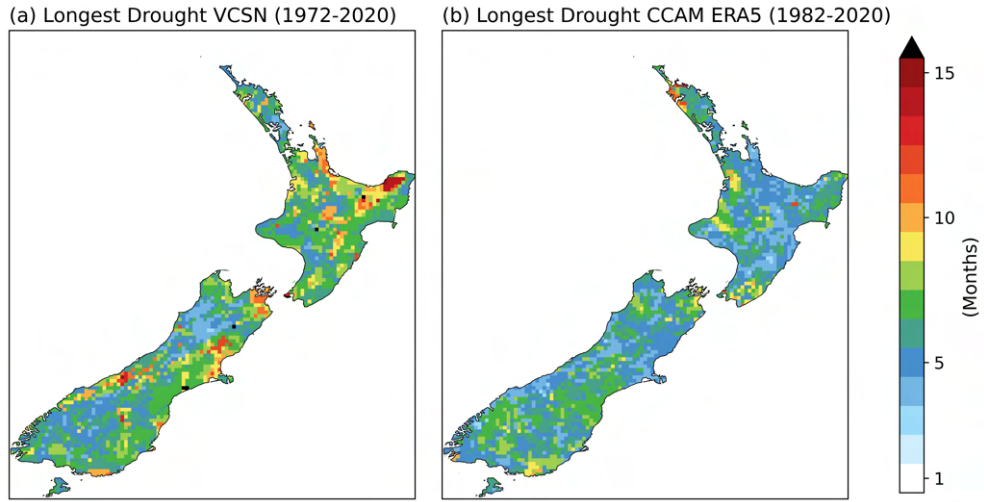

**Fig. S28** Longest droughts present in (a) the VCSN gridded station product for the years 1972-2020, and (b) CCAM downscaled ERA5 for the years 1982-2020.

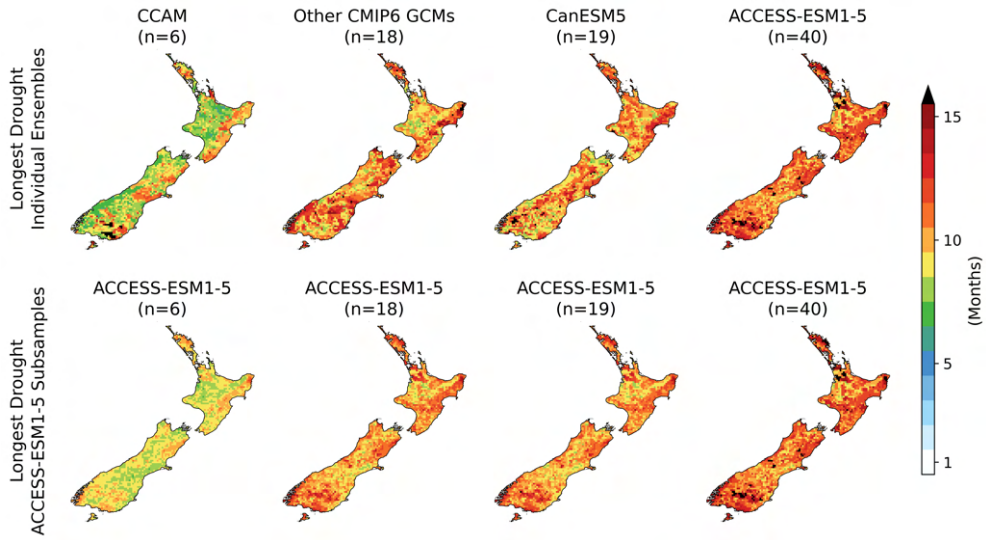

**Fig. S29** First Row: Longest drought across all members of each ensemble at each grid-point within an extended historical period (1965-2014). Second Row: Longest drought within  $n=[6,18,19,40]$  member subsamples of the ACCESS-ESM1-5 ensemble. Subsampling is repeated 100 times and averaged to best represent each subsample size.
